# Supplementary material for: Privacy Preserving Stream Analytics: The Marriage of Randomized Response and Approximate Computing
Source: arXiv:1701.05403 source file (2017-06-05)
Supplement: Supplementary file 1 [file appendix_privacy-eval.tex]

\section{Privacy Analysis Evaluation}
\label{sec:app-privacy-eval}

Figure~\ref{fig:privacy-analysis} depicts the influence any single parameter on the bounds for the two privacy metrics differential privacy and zero\-/knowledge privacy. Subfigures~\ref{fig:epsilonZK-p} to~\ref{fig:epsilonZK-s} represent zero\-/knowledge privacy, while subfigures~\ref{fig:epsilonDP-p} to~\ref{fig:epsilonDP-s} represent the differential privacy metric. The shown results are micro-benchmarks in the sense that the privacy level is calculated using equations~\ref{eq:ezk} and~\ref{eq:edp} with two of the three parameters fixed at specific values and a varying third parameter. The free parameter is~\(p\) from randomize response for figures~\ref{fig:epsilonZK-p} and~\ref{fig:epsilonDP-p} and parameter~\(q\) for figures~\ref{fig:epsilonZK-q} and~\ref{fig:epsilonDP-q}. The influence of the sampling parameter~\(s\) upon the privacy level is plotted in figures~\ref{fig:epsilonZK-s} and~\ref{fig:epsilonDP-s}.

\begin{figure*}[htp]
  \begin{center}
    \subfigure[Relation of \(\epsilon_{zk}\) to parameter \(p\).]{\label{fig:epsilonZK-p}\includegraphics[scale=0.55]{figuresTikZ/eZK_p}}
    \subfigure[Relation of \(\epsilon_{zk}\) to parameter \(q\).]{\label{fig:epsilonZK-q}\includegraphics[scale=0.55]{figuresTikZ/eZK_q}} 
    \subfigure[Relation of \(\epsilon_{zk}\) to parameter \(s\).]{\label{fig:epsilonZK-s}\includegraphics[scale=0.55]{figuresTikZ/eZK_r}}\\   
    \subfigure[Relation of \(\epsilon_{dp}\) to parameter \(p\).]{\label{fig:epsilonDP-p}\includegraphics[scale=0.55]{figuresTikZ/eDP_p}}
    \subfigure[Relation of \(\epsilon_{dp}\) to parameter \(q\).]{\label{fig:epsilonDP-q}\includegraphics[scale=0.55]{figuresTikZ/eDP_q}} 
    \subfigure[Relation of \(\epsilon_{dp}\) to parameter \(s\).]{\label{fig:epsilonDP-s}\includegraphics[scale=0.55]{figuresTikZ/eDP_r}}
  \end{center}
 
  \caption{Privacy analysis of zero-knowledge privacy (\(\epsilon_{zk}\))  and differential privacy  (\(\epsilon_{dp}\)) with different values of $p$, $q$, and $s$}
  
  \label{fig:privacy-analysis}  
\end{figure*}

Zero\-/knowledge privacy and differential privacy describe the advantage \(\epsilon\) of an adversary in learning information about individual \(i\) by using an output from an algorithm running over database \(D\) containing an individual $i \in D$ compared to using a result of possibly another algorithm running over \(D_{-i}\). As the advantage \(\epsilon\) of the adversary is measured identically in both metrics, the privacy levels \(\epsilon_{dp}\) and \(\epsilon_{zk}\) can be compared. Zero\-/knowledge privacy is a strictly stronger privacy metric through the additional usage of external information and access to aggregate information of the remaining database \(D_{-i}\) compared to differential privacy, which is restricted to the same sanitizing algorithm over \(D\) and \(D_{-i}\). One can think of zero\-/knowledge privacy compared to differential privacy as a relaxation on the adversary model, or simply giving the adversary more possibilities. Specifically differential privacy is a special case of zero\-/knowledge privacy when the adversary chooses to use the same algorithm that is used by differential privacy over the remaining database \(D_i\). By intuition as differential privacy is contained within zero\-/knowledge privacy and the adversary aims at maximizing its advantage, tha advantage of an adversary in the zero\-/knowledge model is at least as high and possibly higher than the advantage of an adversary in the differential privacy model: \(\epsilon_{zk} \geq \epsilon_{dp}\). Figure~\ref{fig:epsilonZKbyDP} draws the ratio \(\frac{\epsilon_{zk}}{\epsilon_{dp}}\) between the zero\-/knowledge privacy level \(\epsilon_{zk}\) and the differential privacy level \(\epsilon_{dp}\) given identical values for \(p,q\) and \(s\). Put differently, as the adversary is allowed to do more in the zero\-/knowledge model, the privacy level is lower, which is reflected by a higher \(\epsilon_{zk}\) value compared to the differential privacy level \(\epsilon_{dp}\) --- given identical system parameters.

\begin{figure*}[ht]
  \centering
  \includegraphics[scale=0.8]{figuresTikZ/eZK_eDP} 
  \caption{Ratio of \(\frac{\epsilon_{zk}}{\epsilon_{dp}}\) depending on the sampling parameter \(s\) for different values \(p\) and \(q\).}
  \label{fig:epsilonZKbyDP}
\end{figure*}

%
%\if 0
%
%
%%% Zero-Knowledge Privacy %%
%% Plotted by code/analysis/privacy.r
%\begin{figure}[ht]
%  \centering
%  \includegraphics[width=.35\textwidth]{figuresTikZ/eZK_p}
%  \caption{Relation of \(\epsilon_{zk}\) to parameter \(p\).}
%  \label{fig:epsilonZK-p}
%\end{figure}
%
%% Plotted by code/analysis/privacy.r
%\begin{figure}[ht]
%  \centering
%  \includegraphics[width=.35\textwidth]{figuresTikZ/eZK_q}
%  \caption{Relation of \(\epsilon_{zk}\) to parameter \(q\).}
%  \label{fig:epsilonZK-q}
%\end{figure}
%
%% Plotted by code/analysis/privacy.r
%\begin{figure}[ht]
%  \centering
%  \includegraphics[width=.35\textwidth]{figuresTikZ/eZK_r}
%  \caption{Relation of \(\epsilon_{zk}\) to parameter \(r\).}
%  \label{fig:epsilonZK-r}
%\end{figure}
%
%%% Differential Privacy %%
%% Plotted by code/analysis/privacy.r
%\begin{figure}[ht]
%  \centering
%  \includegraphics[width=.35\textwidth]{figuresTikZ/eDP_p}
%  \caption{Relation of \(\epsilon_{dp}\) to parameter \(p\).}
%  \label{fig:epsilonDP-p}
%\end{figure}
%
%% Plotted by code/analysis/privacy.r
%\begin{figure}[ht]
%  \centering
%  \includegraphics[width=.35\textwidth]{figuresTikZ/eDP_q}
%  \caption{Relation of \(\epsilon_{dp}\) to parameter \(q\).}
%  \label{fig:epsilonDP-q}
%\end{figure}
%
%% Plotted by code/analysis/privacy.r
%\begin{figure}[ht]
%  \centering
%  \includegraphics[width=.35\textwidth]{figuresTikZ/eDP_r}
%  \caption{Relation of \(\epsilon_{dp}\) to parameter \(p\).}
%  \label{fig:epsilonDP-r}
%\end{figure}
%
%\fi 
